# Supplementary material for: An interior-point trust-region method for nonsmooth regularized bound-constrained optimization
Source: arXiv:2402.18423 source file (2024-02-28)
Supplement: Supplementary file 1 [file appendix.tex]

\subsection{Proof 2 (facultative)}
\smarttodo[inline]{Might be redundant with the results from \Cref{sec:convergence-outer}, leaving it here for now just in case.}

The following results are used to show the epi-convergence of the models of the last inner iterations to~\eqref{eq:def-Pbar} at \(\bar x\) for the subsequence \(N\).
This will allow us to perform operations between epi-limits and inferior bounds, which will enable us to establish the convergence of the outer iterations for the subsequence \(N\).

For each \(k \in \N\), the stopping condition of \Cref{alg:bar-inner} occurs in a finite number of iterations.
Let \(\bar{\Delta}_k := \Delta_{\min,k}\) be the minimum radius referred to in the convergence of the inner iterations, and let \(\bar{\nu}_k = \nu_{k,j_k}\), \(\bar{\varphi}_k(s) := \varphi(s; x_{k,j_k})\) and \(\psi_k(s) := \psi(s; x_{k,j_k})\) be the steplength and models of \((f + \phi_k)(x_{k,j+k} + s)\) and \(h(x_{k,j_k} + s)\) employed during the final inner iteration \(j_k\) associated with the \(k\)-th outer iteration.

At iteration \(k\), we get from the previous part that either \(\{(f + \phi_k + h)(x_{k, j})\}_{j = 0}^{\infty}\) is not bounded below, or \(\nu_{k, j_k}^{-1/2} \xi_{\textup{cp}}(\Delta_{k, j_k}; x_{k,j_k}, \nu_{k,j_k})^{1/2} \le \epsilon_{d,k}\).

\begin{shadylemma}
  Under \Cref{asm:liminf-delta-nu}, let \(\bar x\) and \(\bar z\) be limit points of \(\{\bar x_k\}\) and \(\{\bar z_k\}\), respectively.
  Then, there exists a subsequence of \(m_{\textup{cp}}(\cdot; x_{k,j_k}, \nu_{k,j_k}) + \chi(\cdot; \bar \Delta_k \cap \R_{\delta_k}(x_{k,j_k}))\) that epi-converges to a function that is not the infinite function.
\end{shadylemma}
\begin{proof}
  \(\varphi(\cdot; x_{k,j_k}) + \psi(\cdot; x_{k,j_k}) + \tfrac{1}{2}\nu_{k,j}^{-1}\|\cdot\|^2 + \chi(\cdot; \bar \Delta_k \cap \R_{\delta_k}(x_{k,j_k}))\) does not epi-converges to the infinite function since \(\bar \Delta > 0\) and \(\bar \nu > 0\), so we can apply \citep[Theorem~\(7.6\)]{rtrw}.
\end{proof}

\begin{shadylemma}
  \label{lem:elim-chi}
  Let \Cref{asm:liminf-delta-nu} be satisfied, \(\bar x\) and \(\bar z\) be limit points of \(\{\bar x_k\}\) and \(\{\bar z_k\}\), respectively.
  Then, for an infinite subsequence \(N\) such that \(x_{k, j_k} \underset{N}{\rightarrow} \bar x\) with \(\min_i \bar x_i = 0\), there exists \(\tilde \Delta \ge \bar \Delta\) such that
  \begin{equation*}
    e\text{-}\lim_{k \in N} \chi (\cdot; \bar \Delta_{k} \B \cap \R_{\delta_k}(x_{k, j_k})) = \chi (\cdot; \tilde \Delta \B) + \chi(\cdot; (-\bar x + \R_+^n)).
  \end{equation*}
\end{shadylemma}
\begin{proof}
  Using \Cref{asm:liminf-delta-nu}, we have \(\liminf \bar \Delta_k \B = \bar \Delta \B\), and there exists \(\tilde \Delta_1\) and an infinite subsequence \(N_1 \subset N\) such that \(\lim_{N_1} \bar \Delta_k = \tilde \Delta\).
  Now, \(\min_i (x_{k,j_k})_i \underset{N}{\rightarrow} 0\), as \(\bar x\) has at least one component \(i\) such that \(\bar x_i = 0\).
  Then \(\min_i (x_{k,j_k})_i \underset{N}{\rightarrow} 0\), and \(\R_{\delta_k}(x_{k,j_k}) \underset{N}{\rightarrow} (-\bar x + \R_+^n)\).
  Since \(\Delta_k \B\) and \(\R_{\delta_k}(x_{k,j_k})\) are convex (the latter being true because of \Cref{lem:rn-delta-x-convex}) and cannot be separated, we can use \citep[Theorem~\(4.32\)]{rtrw} to conclude that \(\Delta_k \B \cap \R_{\delta_k}(x_{k,j_k}) \underset{N_1}{\rightarrow} \tilde \Delta \B \cap (-\bar x + \R_+^n)\).
  Finally, we use \citep[Theorem~\(7.4f\)]{rtrw} to conclude that \(e\text{-}\lim_{k \in N_1} \chi (\cdot; \bar \Delta_{k} \B \cap \R_{\delta_k}(x_{k, j_k})) = \chi (\cdot; \tilde \Delta \B \cap (-\bar x + \R_+^n)) = \chi (\cdot; \tilde \Delta \B) + \chi(\cdot; (-\bar x + \R_+^n))\).
\end{proof}

To prove the convergence of \Cref{alg:bar-outer}, we want to show that the inner models used in \Cref{alg:bar-inner} approach~\eqref{eq:bar-model}.
This would indicate that our subproblems get closer to the initial problem as \(k\) increases.
To this purpose, we establish the following result, showing the epi-convergence of the objective function of~\eqref{eq:def-model-sub} (up to a constant factor), towards the objective of~\eqref{eq:def-Pbar} (up to a constant factor).
\begin{shadylemma}
  \label{lem:elim-xi}
  Under the assumptions of \Cref{lem:elim-chi}, \Cref{prop:complementarity} and \Cref{asm:psi-epi-continuity}, for an infinite subsequence \(N\) such that \(x_{k, j_k} \underset{N}{\rightarrow} \bar x\) with \(\min_i \bar x_i = 0\), there exists (\(\tilde \Delta \ge \bar \Delta\)) such that
  \begin{multline*}
    e\text{-}\lim_{k \in N} \langle \nabla f(x_{k,j_k}) - z_{k,j_k}; \cdot \rangle + \tfrac{1}{2} \nu_{k,j_k}^{-1} \|\cdot\|^2 + \psi(\cdot; x_{k,j_k}) \\
    + \chi (\cdot; \bar \Delta_{k} \B \cap \R_{\delta_k}(x_{k, j_k})) = \\
    \langle \nabla f(\bar x) - \bar z; \cdot \rangle + \tfrac{1}{2} \bar \nu^{-1} \|\cdot\|^2 + \bar \psi(\cdot; \bar x) + \chi (\cdot; \tilde \Delta \B).
  \end{multline*}
\end{shadylemma}
\begin{proof}
  \Cref{prop:complementarity} and~\eqref{eq:central-path-inner} implies that \(\lim_{k \rightarrow \infty} \|z_{k,j_k} - \mu_k X_{k,j_k}^{-1}e\| = 0\) \smarttodo{Add \cref{asm:kappa-mdb-eps-cv}}, and with~\eqref{eq:z-interval}, we have \(0 \le z_{k, j} \le \kappa_{\textup{zuu}}\) for all \(k\) and \(j\).
  Thus, there exists an infinite subsequence \(\tilde N \subset N\) and \(\bar z \in \R_+^n\) such that \(z_{k,j_k} \underset{k \in \tilde N}{\rightarrow} \bar z\), and \(\mu_k X_{k,j_k}^{-1}e \underset{k \in \tilde N}{\rightarrow} \bar z\).
  We can assume \(\tilde N = N\) without loss of generality.
  Since \(\chi (\cdot; \bar \Delta_{k} \B \cap \R_{\delta_k}(x_{k, j_k}))\), \(\chi (\cdot \mid \tilde \Delta \B)\) and \(\chi(\cdot \mid (-\bar x + \R_+^n))\) are convex, \Cref{lem:elim-chi}, \Cref{asm:liminf-delta-nu} and the fact that \(f\) has a Lipschitz continuous gradient allow us to use \citep[Exercise~\(7.47\)]{rtrw} to establish
  \begin{multline*}
    e\text{-}\lim_{k \in N} \langle \nabla f(x_{k,j_k}) - z_{k,j}; \cdot \rangle + \tfrac{1}{2} \nu_{k,j_k}^{-1} \|\cdot\|^2 + \chi (\cdot; \bar \Delta_{k} \B \cap \R_{\delta_k}(x_{k, j_k})) = \\
    \langle \nabla f(\bar x) - \bar z; \cdot \rangle + \tfrac{1}{2} \bar \nu^{-1} \|\cdot\|^2 + \chi (\cdot; \tilde \Delta \B) + \chi(\cdot; -\bar x + \R_+^n).
  \end{multline*}
  Using \Cref{asm:psi-epi-continuity}, we have \(e\text{-}\lim_{k\in N} \psi(\cdot; x_{k,j_k}) = \psi(\cdot; \bar x)\), and we can use \citep[Theorem~\(7.46\)]{rtrw} to conclude.
\end{proof}

We can now prove the convergence of \Cref{alg:bar-outer}.
\begin{shadytheorem}
  \label{th:xi-cv}
  Under the assumptions of \Cref{lem:elim-chi} \Cref{prop:complementarity} and \Cref{asm:psi-epi-continuity}, \Cref{alg:bar-outer} generates iterates \(x_{k,j_k} \underset{k \in N}{\longrightarrow} \bar x\) such that 
  \begin{equation}
    \liminf_k \xi_{\textup{cp}}(\bar \Delta_k; x_{k,j_k}, \nu_{k,j_k}) = \bar \xi(\tilde \Delta; \bar x, \bar z, \bar \nu) = 0.
  \end{equation}
  Moreover, if the CQ holds at \(\bar x\), then \(\bar x\) a first-order stationary point for~\eqref{eq:nlp}.
\end{shadytheorem}
\begin{proof}
  If there is at least one \(i\) such that \(\bar x_i = 0\), since \(s \mapsto (\nabla f(x_{k, j_k}) - \mu_k X_{k,j_k}^{-1}e)^T s + \tfrac{1}{2} \nu_{k,j_k}^{-1} \|s\|^2 + \psi(s; x_{k, j_k}) + \chi (s; \bar \Delta_{k} \B \cap \R_{\delta_k}(x_{k,j_k}))\) is eventually level-bounded, we can use \Cref{lem:elim-xi} and \Cref{thm:epi-cv-minimization} to conclude that 
  \begin{equation}
    \label{eq:liminf-xi}
    \begin{aligned}
      &\lim_{k \in N} \inf_s (\nabla f(x_{k, j_k}) - \mu_k X_{k,j_k}^{-1}e)^T s + \tfrac{1}{2} \nu_{k,j_k}^{-1} \|s\|^2 + \psi(s; x_{k, j_k})\\
      &\pushright{+ \chi (s; \bar \Delta_{k} \B \cap \R_{\delta_k}(x_{k,j_k}))} \\
      &= \lim_{k \in N} \inf_s m_{\textup{cp}}(s; x_{k,j_k}, \nu_{k,j_k}) - f(x_{k,j_k}) - \phi_k(x_{k,j_k}) + \chi (s; \bar \Delta_{k} \B \cap \R_{\delta_k}(x_{k,j_k}))\\
      &= \inf_s (\nabla f(\bar x)^T - \bar z^T) s + \tfrac{1}{2} \bar \nu^{-1} \|s\|^2 + \bar \psi(s; \bar x) + \chi (s; \tilde \Delta \B)\\
      &= \bar p(\tilde \Delta; \bar x, \bar z, \bar \nu) - f(\bar x),
    \end{aligned}
  \end{equation}
  where we appealed to \Cref{lem:elim-xi} and \Cref{thm:epi-cv-minimization} in the penultimate line.
  We point out that
  \begin{multline*}
    \argmin{s} m_{\textup{cp}}(s; x_{k,j_k}, \nu_{k,j_k}) + \chi (s; \bar \Delta_{k} \B \cap \R_{\delta_k}(x_{k,j_k})) = \\
    \argmin{s} m_{\textup{cp}}(s; x_{k,j_k}, \nu_{k,j_k}) - f(x_{k,j_k}) - \phi_k(x_{k,j_k}) + \chi (s; \bar \Delta_{k} \B \cap \R_{\delta_k}(x_{k,j_k})),
  \end{multline*}
  and
  \begin{equation*}
    \begin{aligned}
      \bar P(\tilde \Delta; \bar x, \bar z, \bar \nu) &= \argmin{s} f(\bar x) + (\nabla f (\bar x)^T - \bar z^T) s + \tfrac{1}{2}\bar \nu^{-1} \|s\|^2 + \bar \psi(s; \bar x) + \chi (s; \tilde \Delta_k \B)\\
      &= \argmin{s} (\nabla f (\bar x)^T - \bar z^T) s + \tfrac{1}{2}\bar \nu^{-1} \|s\|^2 + \bar \psi(s; \bar x) + \chi (s; \tilde \Delta_k \B).
    \end{aligned}
  \end{equation*}
  Therefore, using the second part of \Cref{thm:epi-cv-minimization}, for the sequence
  \begin{equation*}
    s_{k,j_k,1} \in \argmin{s} m_{\textup{cp}}(s; x_{k,j_k}, \nu_{k,j_k}) + \chi (s; \bar \Delta_{k} \B \cap \R_{\delta_k}(x_{k,j_k}))
  \end{equation*}
  and
  \begin{equation*}
    \bar s \in \bar P(\tilde \Delta; \bar x, \bar z, \bar \nu),
  \end{equation*}
  there exists a subsequence \(\bar N \subset \N\) such that
  \begin{equation}
    \label{eq:cv-skj1-bar-s}
    \lim_{k \in \bar N} s_{k,j_k,1} = \bar s.
  \end{equation}
  The epi-limit
  \begin{multline*}
    e\text{-}\lim_{k \in N} \langle \nabla f(x_{k,j_k}) - \mu_k X_{k,j_k}^{-1}e; \cdot \rangle + \psi(\cdot; x_{k,j_k}) + \chi (\cdot; \bar \Delta_{k} \B \cap \R_{\delta_k}(x_{k, j_k})) = \\
    \langle \nabla f(\bar x) - \bar z; \cdot \rangle + \bar \psi(\cdot; \bar x) + \chi (\cdot; \tilde \Delta \B)
  \end{multline*}
  can easily be shown as in \Cref{lem:elim-xi}, because we only removed the term \(\tfrac{1}{2}\nu_{k,j_k}^{-1} \|\cdot\|^2\) whose limit inferior is \(\tfrac{1}{2}\bar \nu^{-1} \|\cdot\|^2\), with \(\bar \nu > 0\).
  Therefore, we have
  \begin{equation*}
    \lim_{k \in N} (\nabla f(x_{k,j_k}) - \mu_k X_{k,j_k}^{-1}e)^T s_{k,j_k,1} + \psi(s_{k,j_k,1}; x_{k,j_k}) = (\nabla f(\bar x)^T - \bar z^T) \bar s + \psi(\bar s; \bar x),
  \end{equation*}
  which leads to
  \begin{equation}
    \label{eq:ineq-xi-epi}
    \begin{aligned}
      &\lim_{k \in \bar N} \xi_{\textup{cp}}(\bar \Delta_k; x_{k,j_k}, \nu_{k,j_k}) \\
      &= \lim_{k \in \bar N} \left( (f + h + \phi_k)(x_{k,j_k}) - \varphi_{\textup{cp}}(s_{k, j_k, 1}; x_{k,j_k}) - \psi(s_{k, j_k, 1}; x_{k,j_k}) \right) \\
      &= \lim_{k \in \bar N} \left(h(x_{k,j_k}) - (\nabla f(x_{k,j_k}) - \mu_k X_{k,j_k}^{-1}e)^T s_{k,j_k,1} - \psi(s_{k,j_k,1}; x_{k,j_k})\right) \\
      &= h(\bar x) - (\nabla f(\bar x)^T - \bar z^T) \bar s - \psi(\bar s; \bar x)\\
      &= \bar \xi(\tilde \Delta; \bar x, \bar z, \bar \nu)\\
      &= 0,
    \end{aligned}
  \end{equation}
  where the last equality is because of \(\epsilon_{d,k} \rightarrow 0\).

  % Now, we recall the expression of \(\bar \xi\)
  % \begin{equation*}
  %   \bar \xi(\bar \Delta_{k}; x_{k, j_k}) = h(x_{k, j_k}) -(\inf_s \nabla f(x_{k, j_k})^T s + \psi(s; x_{k, j_k}) + \chi (s; \bar \Delta_{k} \B \cap (-x_{k,j_k} + \R_+^n))).
  % \end{equation*}
  % Using similar arguments to those of the proof of \Cref{lem:elim-chi}, we can show that 
  % \begin{multline*}
  %   e\text{-}\lim_{k \in N} \langle \nabla f(x_{k,j_k}); \cdot \rangle + \tfrac{1}{2} \nu_{k,j_k}^{-1} \|\cdot\|^2 + \psi(\cdot; x_{k,j_k}) + \chi (\cdot; \bar \Delta_{k} \B \cap ( -x_{k,j_k} + \R_+^n)) = \\
  %   \langle \nabla f(\bar x); \cdot \rangle + \psi(\cdot; \bar x) + \tfrac{1}{2} \bar{\nu}^{-1} \|\cdot\|^2 + \chi (\cdot; \tilde \Delta \B \cap (-\bar x + \R_+^n)).
  % \end{multline*}
  % \smarttodo[inline]{Maybe more details here. Not \(100 \%\) sure the convergence of \(\chi\) is valid but it should be if \((-x_{k,j_k} + \R_+^n) \rightarrow (- \bar x + \R_+^n)\).}
  % We use again \citep[Theorem~\(7.33\)]{rtrw} to establish
  % \begin{multline}
  %   \label{eq:liminf-xi-bar}
  %   \lim_{k \in N} \inf_s \nabla f(x_{k, j_k})^T s + \tfrac{1}{2} \nu_k^{-1} \|s\|^2 + \psi(s; x_{k, j_k}) + \chi (s; \bar \Delta_{k} \B \cap (-x_{k,j_k} + \R_+^n)) = \\
  %   \inf_s  \nabla f(\bar x)^T s + \tfrac{1}{2} \bar{\nu}^{-1} \|s\|^2 + \psi(s; \bar x) + \chi (s; \tilde \Delta \B \cap (-\bar x + \R_+^n)),
  % \end{multline}
  % and for \(s_{k,1} \in \bar P(\bar \Delta_k; x_k, \nu_k)\), there exists a subsequence \(\tilde N \subset \N\) such that \(\lim_{k \in \tilde N} s_{k,1} = \tilde s\), where \(\tilde s \in \bar P(\tilde \Delta; \bar x, \bar \nu)\).

  Now, let us assume that the CQ holds at \(\bar x\).
  For 
  \begin{equation*}
    s_{k,j_k,1} \in \argmin{s} m_{\textup{cp}}(s; x_{k,j_k}, \nu_{k,j_k}) + \chi (s; \bar \Delta_{k} \B \cap \R_{\delta_k}(x_{k,j_k})),
  \end{equation*}
  we have
  \begin{equation}
    \label{eq:epsk-maj-skj1}
    \epsilon_{d,k} \ge \nu_{k,j_k}^{-1/2} \xi_{\textup{cp}}(\bar \Delta_k; x_{k,j_k}, \nu_{k,j_k})^{1/2} \ge \tfrac{1}{2}\nu_{k,j_k}^{-1}\|s_{k,j_k,1}\|,
  \end{equation}
  and \(\liminf \bar \nu_k = \bar \nu > 0\).
  We deduce that \(s_{k,j_k,1} \rightarrow 0\), thus \(\bar s = 0\) using~\eqref{eq:cv-skj1-bar-s}.
  Finally, by applying \Cref{lem:xi-stationarity}, we get \(0 \in \bar P(\tilde \Delta; \bar x, \bar z, \bar \nu)\) and the first-order stationarity of \(\bar x\).

  If there is no \(i\) such that \(\bar x_i = 0\), \(\mu_k X_{k,j_k}^{-1} e \rightarrow 0\), \(\phi_k (x_{k,j_k}) \rightarrow 0\), \(\bar z = 0\), and
  \begin{equation*}
    \begin{aligned}
      &\lim_{k \in N} \inf_s (\nabla f(x_{k, j_k}) - \mu_k X_{k,j_k}^{-1}e)^T s + \tfrac{1}{2} \nu_{k,j_k}^{-1} \|s\|^2 + \psi(s; x_{k, j_k})\\
      &\pushright{+ \chi (s; \bar \Delta_{k} \B \cap \R_{\delta_k}(x_{k,j_k}))} \\
      &= \inf_s \nabla f(\bar x)^T s + \tfrac{1}{2} \bar \nu^{-1} \|s\|^2 + \psi(s; \bar x) + \chi (s; \tilde \Delta \B \cap \R_{\bar \delta}(\bar x)),
    \end{aligned}
  \end{equation*}
  which is analogous to~\eqref{eq:liminf-xi}, can be established by showing the epi-convergence similarly as in \Cref{lem:elim-xi}, and using \Cref{thm:epi-cv-minimization}.\smarttodo{Maybe a bit fast, but I did not want to almost duplicate \Cref{lem:elim-xi}}
  By defining 
  \begin{equation*}
    \bar P_{\mathcal{I}}(\Delta, \delta; x, \nu) = \argmin{s} f(x) + \nabla f(x)^T s + \tfrac{1}{2} \nu^{-1} \|s\|^2 + \psi(s; x) + \chi (s; \Delta \B \cap \R_{\delta}(x)),
  \end{equation*}
  we observe that for some \(0 < \hat \Delta \le \tilde \Delta\) such that \(\hat \Delta \B \subset \tilde \Delta \B \cap \R_{\bar \delta}(\bar x)\), we  have \(0 \in \bar P_{\mathcal{I}}(\tilde \Delta, \bar \delta; \bar x, \bar \nu) \implies 0 \in \bar P(\hat \Delta; \bar x, \bar z, \bar \nu)\).
  Moreover, using again \Cref{thm:epi-cv-minimization}, we get \(s_{k,j_k,1} \rightarrow \bar s \in \bar P_{\mathcal{I}}(\tilde \Delta, \bar \delta; \bar x, \bar \nu)\).
  Using~\eqref{eq:ineq-xi-epi} and~\eqref{eq:epsk-maj-skj1}, we establish that \(\bar s \rightarrow 0\) and use \Cref{lem:xi-stationarity} to conclude that \(\bar x\) is first-order stationary.
\end{proof}

As we pointed out in our remark below \Cref{lem:xi-stationarity}, if \(h\) is convex, then the CQ is not required in \Cref{th:xi-cv}.
